# Supplementary material for: The nature of three-body interactions in DFT: exchange and polarization effects
Source: arXiv:1706.07982 ancillary file (2017-08-10)
Supplement: Supplementary file 1 [file Supp_Mat.pdf]

# Supplementary Information

***to accompany***

**The nature of three-body interactions in DFT: exchange and polarization effects**


Michał Hapka,[1,a)] Łukasz Rajchel,[2,b)] Marcin Modrzejewski,[1] Rainer Schäffer,[2] Grzegorz Chałasiński,[1] and Małgorzata M. Szczęśniak[3]

[1)] *Faculty of Chemistry, University of Warsaw, ul. L. Pasteura 1, 02-093 Warsaw, Poland*

[2)] *Faculty of Chemistry, University of Duisburg-Essen, Universitätsstraße 5, 45117 Essen, Germany*

[3)] *Department of Chemistry, Oakland University, Rochester, Michigan 48309-4477, United States*

[a)] Electronic mail: hapka@tiger.chem.uw.edu.pl

[b)] Electronic mail: L.Rajchel@icm.edu.pl

## I. THE ZEROTH-ORDER EXCHANGE NONADDITIVITY

We begin with the definition, see Eq. (23) in the manuscript:[1] In order to derive the explicit formulas for the Murrell and Lanshoff terms, $\Delta_{\mathrm{M}} + \Delta_{\mathrm{L}}$, let us begin by decomposing the lhs of Eq. (23) in the manuscript into monomer contributions:

$$E_{\mathrm{int}}^{\mathrm{HL}} - E_{\mathrm{int,SAPT}}^{(1)} = \sum_{\mu} \Delta_{\mu}, \tag{S.1}$$

where the monomer contribution is

$$\Delta_{\mu} = \frac{\langle \Phi_0 \,|\, \mathcal{A} H_{\mu} \,|\, \Phi_0 \rangle}{\langle \Phi_0 \,|\, \mathcal{A} \,|\, \Phi_0 \rangle} - \frac{\langle \Psi_{\mu} \,|\, H_{\mu} \,|\, \Psi_{\mu} \rangle}{\langle \Psi_{\mu} \,|\, \Psi_{\mu} \rangle} \tag{S.2}$$

and $\Phi_0 = \Psi_{\mu}\Psi_{\nu} \dots \Psi_L$. Using the partitioning of the monomers' Hamiltionian $\langle \Psi_{\mu} \,|\, H_{\mu} \,|\, \Psi_{\mu} \rangle = \langle \Psi_{\mu} \,|\, F_{\mu} \,|\, \Psi_{\mu} \rangle + \langle \Psi_{\mu} \,|\, W_{\mu} \,|\, \Psi_{\mu} \rangle$ and the norm $\langle \Psi_{\mu} \,|\, \Psi_{\mu} \rangle = 1$ we recast the rhs of Eq. (S.2) using:

$$\frac{\langle \Phi_0 \,|\, \mathcal{A} H_{\mu} \,|\, \Phi_0 \rangle}{\langle \Phi_0 \,|\, \mathcal{A} \,|\, \Phi_0 \rangle} = \frac{\langle \Phi_0 \,|\, \mathcal{A}(F_{\mu} + W_{\mu}) \,|\, \Phi_0 \rangle}{\langle \Phi_0 \,|\, \mathcal{A} \,|\, \Phi_0 \rangle} \tag{S.3}$$

and

$$\frac{\langle \Psi_{\mu} \,|\, H_{\mu} \,|\, \Psi_{\mu} \rangle}{\langle \Psi_{\mu} \,|\, \Psi_{\mu} \rangle} = \Big( \langle \Psi_{\mu} \,|\, F_{\mu} \,|\, \Psi_{\mu} \rangle + \langle \Psi_{\mu} \,|\, W_{\mu} \,|\, \Psi_{\mu} \rangle \Big) \frac{\langle \Phi_0 \,|\, \mathcal{A} \,|\, \Phi_0 \rangle}{\langle \Phi_0 \,|\, \mathcal{A} \,|\, \Phi_0 \rangle}. \tag{S.4}$$

This leads to the partitioning of $\Delta_{\mu}$ into the Landshoff and Murrell terms:

$$\begin{aligned} \Delta_{\mu} &= \frac{\Big\langle \Phi_0 \,\Big|\, \mathcal{A}\Big(F_{\mu} - \langle \Psi_{\mu} \,|\, F_{\mu} \,|\, \Psi_{\mu} \rangle\Big) \,\Big|\, \Phi_0 \Big\rangle}{\langle \Phi_0 \,|\, \mathcal{A} \,|\, \Phi_0 \rangle} + \frac{\Big\langle \Phi_0 \,\Big|\, \mathcal{A}\Big(W_{\mu} - \langle \Psi_{\mu} \,|\, W_{\mu} \,|\, \Psi_{\mu} \rangle\Big) \,\Big|\, \Phi_0 \Big\rangle}{\langle \Phi_0 \,|\, \mathcal{A} \,|\, \Phi_0 \rangle} \\ &= \Delta_{\mathrm{L}}^{\mu} + \Delta_{\mathrm{M}}^{\mu}. \end{aligned} \tag{S.5}$$

The explicit formula for the $\Delta_{\mathrm{M}}^{\mu}$ term reads:[1]

$$\Delta_{\mathrm{M}}^{\mu} = \frac{1}{2} \iint \frac{\rho_{\mathrm{exch}}^{\mu}(k)\rho_{\mathrm{exch}}^{\mu}(l) - \rho_{\mathrm{exch}}^{\mu}(k|l)\rho_{\mathrm{exch}}^{\mu}(l|k)}{r_{kl}} \mathrm{d}k\mathrm{d}l, \tag{S.6}$$

where $\rho_{\mathrm{exch}}^{\mathrm{A}}(k'|k)$ is the exchange contribution to the first-order interaction density matrix:

$$\rho_{\mathrm{exch}}^{\mathrm{A}}(k'|k) = 2 \sum_{p \in A} \sum_{r} P_{rp} \varphi_p^*(k') \varphi_r(k). \tag{S.7}$$

(We use the same notation as in Ref. 1.) The **P** matrix is defined as

$$\mathbf{P} = \mathbf{S}(\mathbf{1} + \mathbf{S})^{-1}, \tag{S.8}$$

with **S** denoting the matrix of intermolecular overlap integrals between occupied monomer orbitals $S_{ij} = \langle \varphi_i | \varphi_j \rangle$. The first part of (S.6) gives:

$$\begin{aligned} \iint \frac{\rho_{\mathrm{exch}}^{\mathrm{A}}(k)\rho_{\mathrm{exch}}^{\mathrm{A}}(l)}{r_{kl}} dkdl &= 4 \sum_{p,q \in A} \sum_{r,s} P_{rp} P_{sq} \iint \frac{\varphi_p^*(k)\varphi_r(k)\varphi_q^*(l)\varphi_s(l)}{r_{kl}} dldk \\ &= 4 \sum_{p,q \in A} \sum_{r,s} P_{rp} P_{sq} (pr|qs) = 4 \sum_{p,q \in A} \sum_{r,s} P_{rp} P_{sq} (rp|sq), \end{aligned} \tag{S.9}$$

while the second part gives:

$$\iint \frac{\rho^{\rm A}_{\rm exch}(k|l)\rho^{\rm A}_{\rm exch}(l|k)}{r_{kl}} dkdl = 4\sum_{p,q\in A}\sum_{r,s} P_{rp}P_{sq} \iint \frac{\varphi_p^*(k)\varphi_s(k)\varphi_q^*(l)\varphi_r(l)}{r_{kl}} dldk$$
$$= 4\sum_{p,q\in A}\sum_{r,s} P_{rp}P_{sq}(ps|qr). \tag{S.10}$$

Using (S.9) and (S.10) we can give formulas in the AO basis. For the AB dimer the $\Delta_{\rm M}$ term takes the form:

$$\Delta^{\rm AB}_{\rm M} = 4{\rm Tr}\Big((\mathbf{P}^{\rm A}+\mathbf{P}^{\rm AB})\big(\mathbf{J}[\mathbf{P}^{\rm A}]+\mathbf{J}[\mathbf{P}^{\rm BA}]-\mathbf{K}[\mathbf{P}^{\rm A}]-\mathbf{K}[\mathbf{P}^{\rm BA}]\big)\Big)$$
$$+ 4{\rm Tr}\Big((\mathbf{P}^{\rm B}+\mathbf{P}^{\rm AB})\big(\mathbf{J}[\mathbf{P}^{\rm B}]+\mathbf{J}[\mathbf{P}^{\rm BA}]-\mathbf{K}[\mathbf{P}^{\rm B}]-\mathbf{K}[\mathbf{P}^{\rm BA}]\big)\Big) \tag{S.11}$$

while for the ABC trimer :

$$\Delta^{\rm ABC}_{\rm M} = 4{\rm Tr}\Big((\mathbf{P}^{\rm A}+\mathbf{P}^{\rm AB}+\mathbf{P}^{\rm AC})\big(\mathbf{J}[\mathbf{P}^{\rm A}]+\mathbf{J}[\mathbf{P}^{\rm BA}]+\mathbf{J}[\mathbf{P}^{\rm CA}]-\mathbf{K}[\mathbf{P}^{\rm A}]-\mathbf{K}[\mathbf{P}^{\rm BA}]-\mathbf{K}[\mathbf{P}^{\rm CA}]\big)\Big)$$
$$+ 4{\rm Tr}\Big((\mathbf{P}^{\rm B}+\mathbf{P}^{\rm AB}+\mathbf{P}^{\rm CB})\big(\mathbf{J}[\mathbf{P}^{\rm B}]+\mathbf{J}[\mathbf{P}^{\rm BA}]+\mathbf{J}[\mathbf{P}^{\rm BC}]-\mathbf{K}[\mathbf{P}^{\rm B}]-\mathbf{K}[\mathbf{P}^{\rm BA}]-\mathbf{K}[\mathbf{P}^{\rm BC}]\big)\Big)$$
$$+ 4{\rm Tr}\Big((\mathbf{P}^{\rm C}+\mathbf{P}^{\rm AC}+\mathbf{P}^{\rm BC})\big(\mathbf{J}[\mathbf{P}^{\rm C}]+\mathbf{J}[\mathbf{P}^{\rm CA}]+\mathbf{J}[\mathbf{P}^{\rm CB}]-\mathbf{K}[\mathbf{P}^{\rm B}]-\mathbf{K}[\mathbf{P}^{\rm BA}]-\mathbf{K}[\mathbf{P}^{\rm BC}]\big)\Big) \tag{S.12}$$

In the above expressions $\mathbf{P}^{XY}$ matrix is transformed to the AO basis:

$$\mathbf{P}^{XY} = (\mathbf{C}^X)^\dagger\big([\mathbf{S}+\mathbf{1}]^{-1}-\mathbf{1}\big)\mathbf{C}^Y, \tag{S.13}$$

while $\mathbf{J}[X]$ and $\mathbf{K}[X]$ denote the generalized Coulomb and exchange matrices:

$$J[X]_{\mu\nu} = \frac{1}{2}\sum_{\lambda\sigma} X_{\lambda\sigma}(\mu\nu|\lambda\sigma)$$
$$K[X]_{\mu\nu} = \frac{1}{2}\sum_{\lambda\sigma} X_{\lambda\sigma}(\mu\lambda|\sigma\nu) \tag{S.14}$$

Finally, we calculate the zeroth-order exchange-nonadditivity, $\Delta_{\rm M}$, as the difference between the three-body and two-body contributions:

$$\Delta_{\rm M} = \Delta^{\rm ABC}_{\rm M} - \Delta^{\rm AB}_{\rm M} - \Delta^{\rm BC}_{\rm M} - \Delta^{\rm AC}_{\rm M}. \tag{S.15}$$

## II. PAULI BLOCKADE FORMALISM FOR MANY-BODY SYSTEMS

Below we outline the basic equations of the PB[2] and PBdf[3] schemes generalized for a system composed of $L$ weakly interacting monomers (denoted $\mu, \nu, \ldots$). The total Hamiltonian of the system is a sum of monomer Hamiltonians and the interaction part,

$$\hat{H} = \sum_{\mu=1}^{L} \hat{H}_\mu + \sum_{\mu=1}^{L-1}\sum_{\nu=\mu+1}^{L} V_{\mu\nu} \tag{S.16}$$
$$= \hat{H}_0 + V_{\rm int}. \tag{S.17}$$

Before the PB computation we solve the standard KS equations for each isolated monomer.

In the zeroth iteration of the PB iterative process, we enforce the orthogonality of the occupied orbitals

$$\left\langle \tilde{\varphi}_\mu^i \,\middle|\, \tilde{\varphi}_\nu^j \right\rangle = \delta_{\mu\nu}\delta_{ij}, \tag{S.18}$$

where the lower index labels the monomer and the upper index is the occupied orbital index within the monomer. In our implementation we use the symmetric Löwdin scheme[4].

The single-determinantal wave function of the complex built from the orthogonal orbitals is $\tilde{\Phi}$ and the corresponding density reads

$$\begin{aligned} \rho &= \left\langle \tilde{\Phi} \,\middle|\, \hat{\rho} \,\middle|\, \tilde{\Phi} \right\rangle \\ &= \sum_{\mu=1}^{L} \left\langle \tilde{\Phi}_\mu \,\middle|\, \hat{\rho}_\mu \,\middle|\, \tilde{\Phi}_\mu \right\rangle \\ &= \sum_{\mu=1}^{L} \tilde{\rho}_\mu. \end{aligned} \tag{S.19}$$

The total energy of the cluster is

$$\begin{aligned} E[\tilde{\rho}_1, \tilde{\rho}_2, \ldots, \tilde{\rho}_L] = &\sum_{\mu=1}^{L} E_\mu[\tilde{\rho}_\mu] \\ &+ \sum_{\mu=1}^{L-1} \sum_{\nu=\mu+1}^{L} E_{\text{elst}}[\tilde{\rho}_\mu, \tilde{\rho}_\nu] + \Delta E_{\text{xc}}[\tilde{\rho}_1, \tilde{\rho}_2, \ldots; \tilde{\rho}_L], \end{aligned} \tag{S.20}$$

where $E_\mu[\tilde{\rho}_\mu]$ is the monomer energy functional, the electrostatic interaction term reads

$$\begin{aligned} E_{\text{elst}}[\tilde{\rho}_\mu, \tilde{\rho}_\nu] = &\int_{\mathbb{R}^3} v_\nu(\mathbf{r})\tilde{\rho}_\mu(\mathbf{r})\, \mathrm{d}^3\mathbf{r} + \int_{\mathbb{R}^3} v_\mu(\mathbf{r})\tilde{\rho}_\nu(\mathbf{r})\, \mathrm{d}^3\mathbf{r} \\ &+ \int_{\mathbb{R}^3}\int_{\mathbb{R}^3} \frac{\tilde{\rho}_\mu(\mathbf{r}_1)\tilde{\rho}_\nu(\mathbf{r}_1)}{r_{12}} \mathrm{d}^3\mathbf{r}_1\, \mathrm{d}^3\mathbf{r}_2 + W_{\mu\nu}, \end{aligned} \tag{S.21}$$

with $W_{\mu\nu}$ denoting the nuclear-nuclear repulsion energy, and the xc energy nonadditivity is

$$\Delta E_{\text{xc}}[\tilde{\rho}_1, \tilde{\rho}_2, \ldots, \tilde{\rho}_L] = E^{\text{xc}}[\rho] - \sum_{\mu=1}^{L} E^{\text{xc}}[\tilde{\rho}_\mu]. \tag{S.22}$$

The total energy is minimized with respect to monomer densities obtained from the orbitals solving a set of $L$ monomer Kohn-Sham equations[2]

$$\left( f_\mu(\mathbf{r}) + \sum_{\nu\neq\mu}^{L} \Big( v_\nu(\mathbf{r}) + j_\nu(\mathbf{r}) \Big) + v^{\text{xc}}(\mathbf{r}) - v_\mu^{\text{xc}}(\mathbf{r}) \right) \tilde{\varphi}_\mu^i(\mathbf{r}) = \epsilon_\mu^i \tilde{\varphi}_\mu^i(\mathbf{r}), \tag{S.23}$$

where $v_\mu(\mathbf{r})$ is a nuclei-electron attraction, $j_\mu(\mathbf{r})$ is the Coulomb electron-electron repulsion, and $v_\mu^{\text{xc}}(\mathbf{r})$ is the exchange-correlation (xc) potential. Eq. (S.23) is solved in an iterative fashion keeping the monomers' orbitals orthogonal at all times. This may be achieved either with the use of the penalty function[2], or the exponential ansatz of orbital rotation.[5] The latter scheme is

more efficient and numerically stable, and therefore has been used in the current implementation of the PB method.

Let the densities of the unperturbed monomers be $\rho_\mu$. The interaction energy is then computed with a supermolecular expression,

$$E_{\mathrm{int}}[\tilde{\rho}_1, \tilde{\rho}_2, \ldots, \tilde{\rho}_L] = E[\tilde{\rho}_1, \tilde{\rho}_2, \ldots, \tilde{\rho}_L] - \sum_{\mu=1}^{L} E_\mu\left[\rho_\mu\right] \tag{S.24}$$

$$= \sum_{\mu=1}^{L-1} \sum_{\nu=\mu+1}^{L} E_{\mathrm{elst}}[\tilde{\rho}_\mu, \tilde{\rho}_\nu] + \Delta E_{\mathrm{xc}}[\tilde{\rho}_1, \tilde{\rho}_2, \ldots, \tilde{\rho}_L] + \sum_{\mu=1}^{L} \Delta E_\mu[\tilde{\rho}_\mu], \tag{S.25}$$

where

$$\Delta E_\mu[\tilde{\rho}_\mu] = E_\mu[\tilde{\rho}_\mu] - E_\mu\left[\rho_\mu\right] \tag{S.26}$$

is the energy effect of orbital orthogonalization. The PB scheme restores the supermolecular KS interaction energy.

The dispersion-free approximation, i.e. the PBdf scheme, is obtained from Eq. (S.20) through replacement of the xc nonadditivity, $\Delta E_{\mathrm{xc}}$, with the exact exchange energy:

$$\begin{aligned} E^{\mathrm{dfree}}[\tilde{\rho}_1, \tilde{\rho}_2, \ldots, \tilde{\rho}_L] = &\sum_{\mu=1}^{L} E_\mu[\tilde{\rho}_\mu] \\ &+ \sum_{\mu=1}^{L-1} \sum_{\nu=\mu+1}^{L} \Big( E_{\mathrm{elst}}[\tilde{\rho}_\mu, \tilde{\rho}_\nu] + E_{\mathrm{exch}}[\tilde{\rho}_\mu, \tilde{\rho}_\nu] \Big) \end{aligned} \tag{S.27}$$

where $E_{\mathrm{exch}}$ is given by the HF formula.

The minimization of Eq. (S.27) yields equations for optimum orbitals,

$$\left( f_\mu(\mathbf{r}) + \sum_{\nu \neq \mu}^{L} \Big( v_\nu(\mathbf{r}) + j_\nu(\mathbf{r}) - k_\nu(\mathbf{r}) \Big) \right) \tilde{\varphi}_\mu^i(\mathbf{r}) = \epsilon_\mu^i \tilde{\varphi}_\mu^i(\mathbf{r}), \tag{S.28}$$

where $k_\nu(\mathbf{r})$ is an exact exchange operator. The orthogonality of the monomer orbitals in Eq. (S.28) is enforced in the same way as in the full PB scheme. The Eqs. (S.28) have a clear physical interpretation, schematically presented for $L = 3$ in Fig. 1. Interacting monomers are described with the full KS operators and the interaction with the other monomers is represented solely by the HF Coulomb and exchange operators. This is why the method is referred to as *dispersion-free*: the intramonomer correlation is included at the KS level, while the intermonomer correlation is deliberately omitted.

The interaction energy in the PB scheme is again computed in a supermolecular way,

$$E_{\mathrm{int}}^{\mathrm{dfree}}[\tilde{\rho}_1, \tilde{\rho}_2, \ldots, \tilde{\rho}_L] = E^{\mathrm{dfree}}[\tilde{\rho}_1, \tilde{\rho}_2, \ldots, \tilde{\rho}_L] - \sum_{\mu=1}^{L} E_\mu\left[\rho_\mu\right] \tag{S.29}$$

$$= \sum_{\mu=1}^{L-1} \sum_{\nu=\mu+1}^{L} \Big( E_{\mathrm{elst}}[\tilde{\rho}_\mu, \tilde{\rho}_\nu] + E_{\mathrm{exch}}[\tilde{\rho}_\mu, \tilde{\rho}_\nu] \Big) + \sum_{\mu=1}^{L} \Delta E_\mu[\tilde{\rho}_\mu]. \tag{S.30}$$

Note that the zero-iteration interaction energy of Eq. (S.30) is equal to the $E^{\rm dfree}_{\rm nadd-ex}$ term.[2] To get the total interaction energy, Eq. (S.30) needs to be supplemented with the assorted dispersion terms, e.g. from SAPT.

## III. ADDITIONAL RESULTS

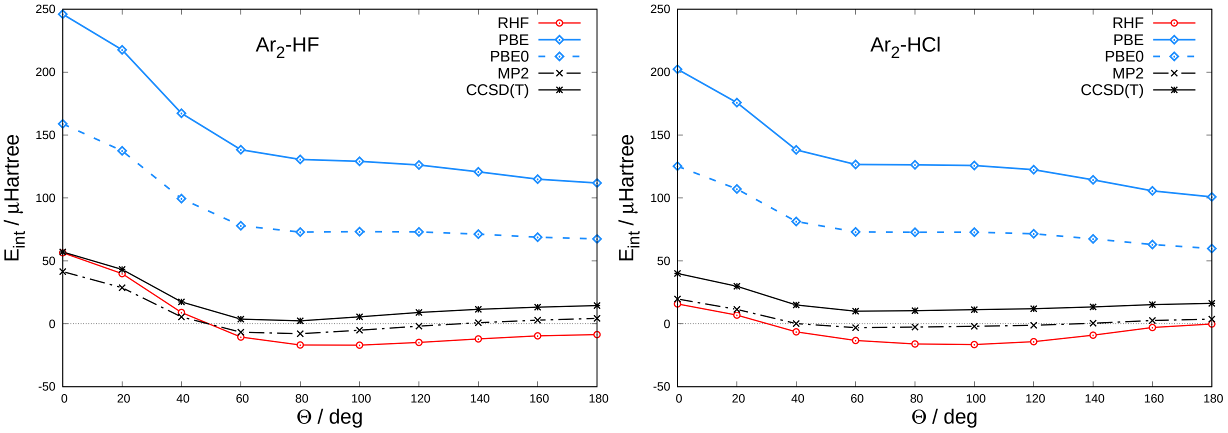


FIG. S1. Three-body nonadditive interaction energy ($\mu$Hartree) for the in-plane bend of the $Ar_2$-HF and $Ar_2$-HCl trimers: comparison of PBE, PBE0 with *ab initio* results.

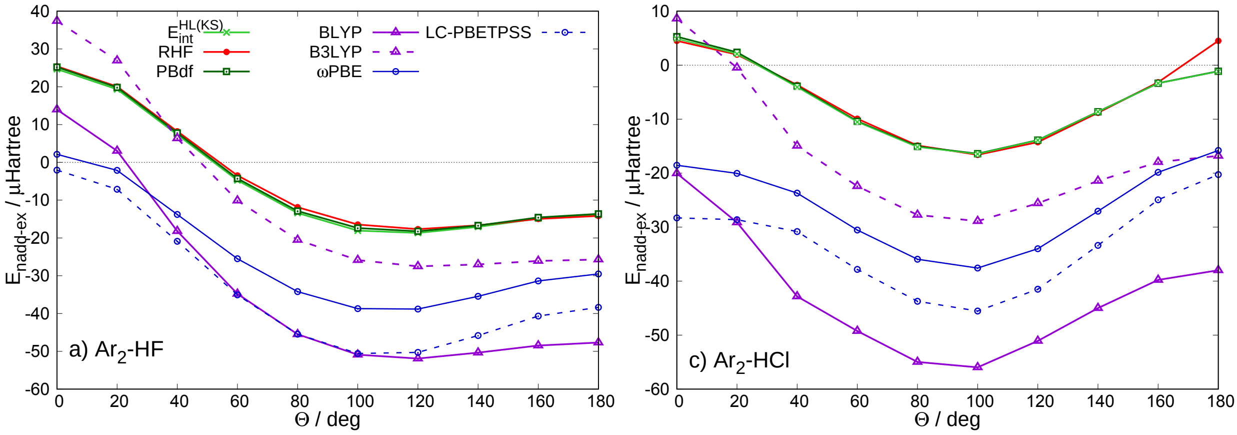


FIG. S2. Three-body nonadditive exchange energy $E_{\rm nadd-ex}$ ($\mu$Hartree) for the in-plane bend of $Ar_2$-HF and $Ar_2$-HCl.

TABLE S1. Nonadditive exchange energies ($\mu$Hartree) for $He_3$, $Ar_3$, $Ar_2$-HF and $Ar_2$-HCl systems obtained with different DFAs (AC denotes the Fermi-Amaldi-Tozer-Handy asymptotic correction[6,7]). The $E^{(1)}_{\rm exch,SAPT}(S^2+S^3+S^4)$ component was calculated in the SAPT2012 program.[8] The following basis sets were used: d-aug-cc-pV5Z for $He_3$,[9] aug-cc-pVQZ for $Ar_3$ and aug-cc-pVTZ[10] for both $Ar_2$-HF and $Ar_2$-HCl. See the manuscript for geometries.

| | | BLYP | **BLYPAC** | PBE | **PBEAC** | B3LYP | **B3LYPAC** | BHLYP | **BHLYPAC** | PBE0 | **PBE0AC** | RHF |
|---|---|---|---|---|---|---|---|---|---|---|---|---|
| $He_3$ | $E^{(1)}_{\rm exch,SAPT}(S^2+S^3+S^4)$ | -2.739 | -0.985 | -2.622 | -0.983 | -1.999 | -0.962 | -1.342 | -0.925 | -1.777 | -0.946 | -0.785 |
| ($R=5.6$ a$_0$) | $\Delta_{\rm M}$ | 0.040 | 0.010 | 0.037 | 0.011 | 0.027 | 0.009 | 0.017 | 0.010 | 0.023 | 0.010 | 0.008 |
| | $E^{\rm HL(KS)}_{\rm int}$ | -2.699 | **-0.975** | -2.585 | **-0.972** | -1.972 | **-0.952** | -1.326 | **-0.916** | -1.754 | **-0.936** | -0.777 |
| $Ar_3$ | $E^{(1)}_{\rm exch,SAPT}(S^2+S^3+S^4)$ | -29.50 | -27.65 | -26.25 | -24.84 | -24.60 | -23.61 | -20.39 | -20.10 | -21.15 | -20.53 | -17.09 |
| ($R=7.0$ a$_0$) | $\Delta_{\rm M}$ | 5.571 | 3.698 | 4.741 | 3.425 | 4.445 | 3.356 | 3.540 | 3.217 | 3.615 | 3.009 | 2.776 |
| | $E^{\rm HL(KS)}_{\rm int}$ | -23.93 | **-23.96** | -21.50 | **-21.42** | -20.16 | **-20.26** | -16.85 | **-16.88** | -17.53 | **-17.52** | -14.31 |
| $Ar_2$-HF | $E^{(1)}_{\rm exch,SAPT}(S^2+S^3+S^4)$ | 20.86 | 24.64 | 19.64 | 22.80 | 20.90 | 22.94 | 21.09 | 21.45 | 19.47 | 20.81 | 23.83 |
| ($\Theta=0°$) | $\Delta_{\rm M}$ | 5.571 | 3.698 | 4.741 | 3.425 | 4.445 | 3.356 | 3.540 | 3.217 | 3.615 | 3.009 | 2.776 |
| | $E^{\rm HL(KS)}_{\rm int}$ | 25.82 | **27.74** | 23.94 | **25.70** | 24.65 | **25.69** | 23.85 | **24.04** | 22.52 | **23.31** | 25.75 |
| $Ar_2$-HCl | $E^{(1)}_{\rm exch,SAPT}(S^2+S^3+S^4)$ | -2.215 | -0.281 | -0.418 | 1.025 | -0.110 | 0.949 | 1.535 | 1.858 | 1.398 | 2.047 | 2.286 |
| ($\Theta=0°$) | $\Delta_{\rm M}$ | 5.143 | 3.515 | 4.370 | 3.263 | 4.116 | 3.187 | 3.283 | 3.037 | 3.341 | 2.861 | 2.583 |
| | $E^{\rm HL(KS)}_{\rm int}$ | 2.929 | **3.234** | 3.951 | **4.288** | 4.005 | **4.136** | 4.818 | **4.895** | 4.739 | **4.907** | 4.870 |

TABLE S2. Nonadditive exchange energies ($\mu$Hartree) for the $He_3$ system at equilateral triangle geometries (d5z basis). In DFT-SAPT calculations PBE0AC the functional was used. PBdf results were obtained with $\omega$PBE and PBE0 functionals. Distance given in bohr.

| $R$ | HF | KS | | | | |
|---|---|---|---|---|---|---|
| | $E^{\text{dfree}}_{\text{nadd-ex}}$ | $E^{(1)}_{\text{exch,SAPT}}$ | $\Delta_{\text{M}}$ | $E^{\text{HL(KS)}}_{\text{int}}$ | $E^{\text{dfree}}_{\text{nadd-ex}}$ ($\omega$PBE) | $E^{\text{dfree}}_{\text{nadd-ex}}$ (PBE0) |
| 4.0 | −186.3 | −213.2 | 8.263 | −204.9 | −195.3 | −240.8 |
| 5.0 | −6.327 | −7.073 | 0.136 | −6.937 | −6.796 | −9.952 |
| 5.6 | −0.778 | −0.859 | 0.010 | −0.849 | −0.847 | −1.390 |
| 6 | −0.189 | −0.205 | 0.002 | −0.203 | −0.207 | −0.368 |

TABLE S3. Nonadditive exchange energies ($\mu$Hartree) for the $Ar_3$ system at equilateral triangle geometries (aug-cc-pVQZ basis). In DFT-SAPT calculations PBE0AC the functional was used. PBdf results were obtained with $\omega$PBE and PBE0 functionals. Distance given in bohr.

| $R$ | HF | KS | | | | |
|---|---|---|---|---|---|---|
| | $E^{\text{dfree}}_{\text{nadd-ex}}$ | $E^{(1)}_{\text{exch,SAPT}}$ | $\Delta_{\text{M}}$ | $E^{\text{HL(KS)}}_{\text{int}}$ | $E^{\text{dfree}}_{\text{nadd-ex}}$ ($\omega$PBE) | $E^{\text{dfree}}_{\text{nadd-ex}}$ (PBE0) |
| 6.0 | −208.7 | −278.2 | 68.74 | −209.4 | −210.8 | −197.0 |
| 7.0 | −14.35 | −17.50 | 3.009 | −14.49 | −14.87 | −14.75 |
| 7.5 | −3.628 | −4.269 | 0.581 | −3.688 | −3.799 | −3.914 |
| 8.0 | −0.900 | −1.021 | 0.108 | −0.913 | −0.951 | −1.022 |

TABLE S4. First-order SAPT and PBdf three-body exchange nonadditivity (kcal/mol) for the $H_2O$ trimers in 1a-c geometries of Ref. 11 (PBE0AC, aug-cc-pVQZ). $E^{\text{HL(KS)}}_{\text{int}}$ is defined as $E^{(1)}_{\text{exch,SAPT}} + \Delta_{\text{M}}$. Additionally, second-order coupled exchange-dispersion energies $E^{(2)}_{\text{exch-disp}}$ at SAPT(PBE0AC) level of theory are given.

| $H_2O$ | HF | KS | | | | |
|---|---|---|---|---|---|---|
| | $E^{\text{dfree}}_{\text{nadd-ex}}$ | $E^{(1)}_{\text{exch,SAPT}}$ | $\Delta_{\text{M}}$ | $E^{\text{HL(KS)}}_{\text{int}}$ | $E^{\text{dfree}}_{\text{nadd-ex}}$ | $E^{(2)}_{\text{exch-disp}}$ |
| 1a | −0.063 | −0.231 | 0.174 | −0.057 | −0.056 | 0.025 |
| 1b | −0.132 | −0.302 | 0.179 | −0.123 | −0.119 | 0.046 |
| 1c | −0.286 | −0.609 | 0.307 | −0.302 | −0.255 | 0.196 |

TABLE S5. Three-body exchange, Murrell delta, and second-order exchange-dispersion energy contributions obtained at DFT-SAPT level of theory with the PBE0AC functional. The basis set was aug-cc-pVQZ. All energies in $\mu$Hartree. $E^{(2)}_{\rm exch-disp}$ and $E^{(2)*}_{\rm exch-disp}$ denote coupled and uncoupled Kohn-Sham exchange-dispersion energies, respectively. See also Figs. S6 and S3.

| | $Ar_2$-HF | | | | $Ar_2$-HCl | | | |
|---|---|---|---|---|---|---|---|---|
| $\Theta$ | $E^{(1)}_{\rm exch}$ | $\Delta_{\rm M}$ | $E^{(2)}_{\rm exch-disp}$ | $E^{(2)*}_{\rm exch-disp}$ | $E^{(1)}_{\rm exch}$ | $\Delta_{\rm M}$ | $E^{(2)}_{\rm exch-disp}$ | $E^{(2)*}_{\rm exch-disp}$ |
| 0 | 22.175 | 2.500 | 12.300 | 14.681 | 2.038 | 2.854 | 18.336 | 22.089 |
| 20 | 16.802 | 2.537 | 11.908 | 13.977 | -0.873 | 2.952 | 16.953 | 20.204 |
| 40 | 4.876 | 2.449 | 11.234 | 12.735 | -6.876 | 2.809 | 14.585 | 17.070 |
| 60 | -6.798 | 2.064 | 10.987 | 12.172 | -12.715 | 2.190 | 13.665 | 15.898 |
| 80 | -15.018 | 1.623 | 11.152 | 12.291 | -16.843 | 1.675 | 13.917 | 16.158 |
| 100 | -19.219 | 1.339 | 11.282 | 12.440 | -17.878 | 1.425 | 13.702 | 15.888 |
| 120 | -19.854 | 1.181 | 10.915 | 12.053 | -15.150 | 1.253 | 12.430 | 14.459 |
| 140 | -18.147 | 1.090 | 10.081 | 11.178 | -9.725 | 1.098 | 10.403 | 12.238 |
| 160 | -15.924 | 1.046 | 9.241 | 10.303 | -4.365 | 1.000 | 8.463 | 10.146 |
| 180 | -14.936 | 1.035 | 8.897 | 9.945 | -2.129 | 0.970 | 7.656 | 9.283 |

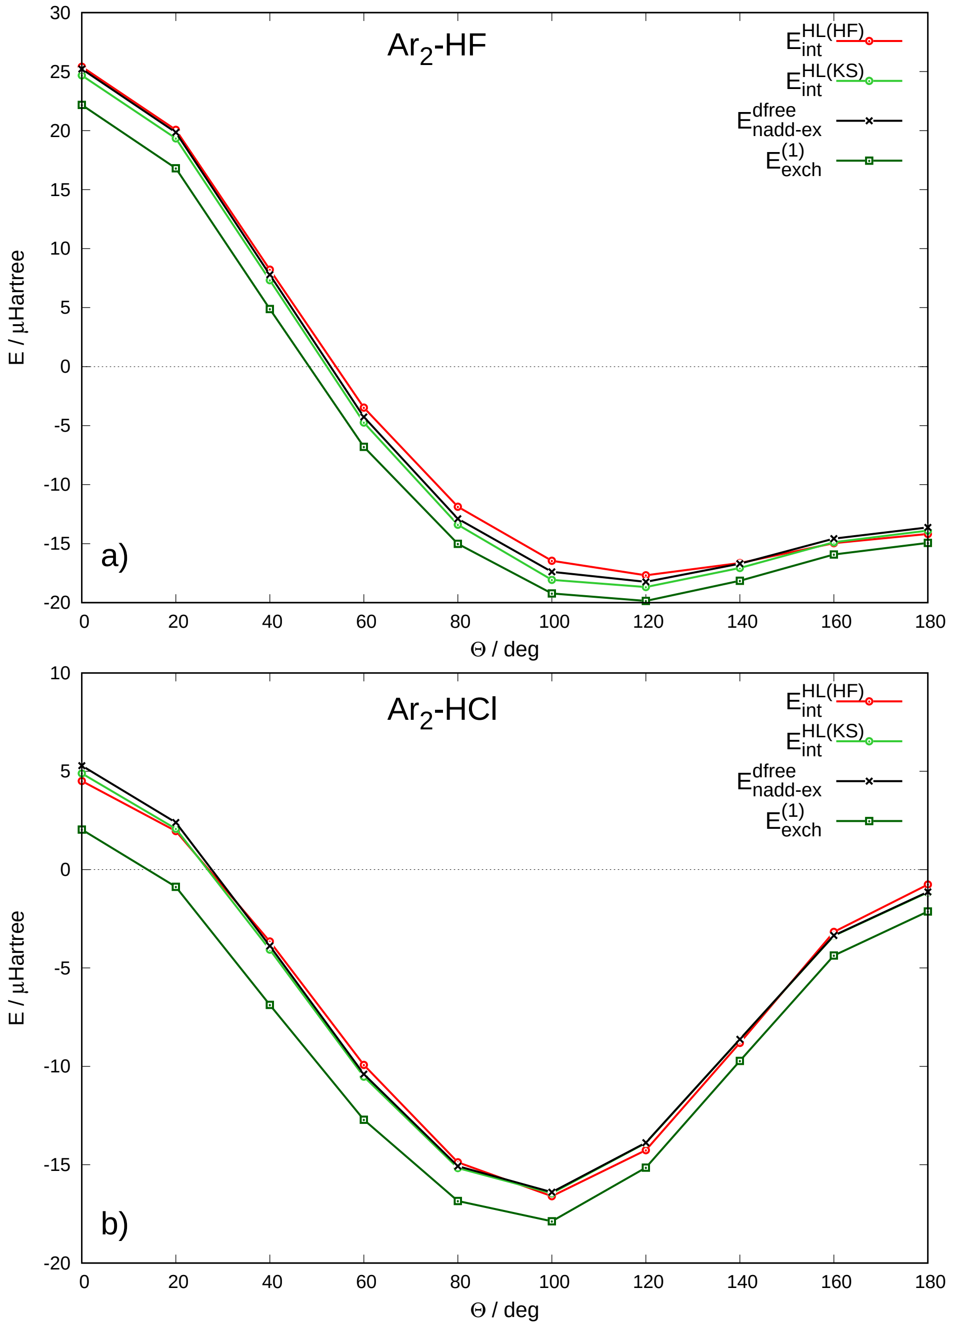


FIG. S3. Three-body nonadditive exchange energy for the in-plane bend of the a) $Ar_2$-HF, b) $Ar_2$-HCl clusters. $E_{\mathrm{int}}^{\mathrm{HL(HF)}}$ and $E_{\mathrm{int}}^{\mathrm{HL(KS)}}$ denote the Hartree-Fock and Kohn-Sham nonadditive Heitler-London interaction energies, respectively, $E_{\mathrm{nadd-ex}}^{\mathrm{dfree}}$ are the PBdf results, $E_{\mathrm{exch}}^{(1)}$ is the DFT-SAPT exchange. In DFT-SAPT and PBdf calculations the PBE0AC functional was used. The basis set was aug-cc-pVQZ.

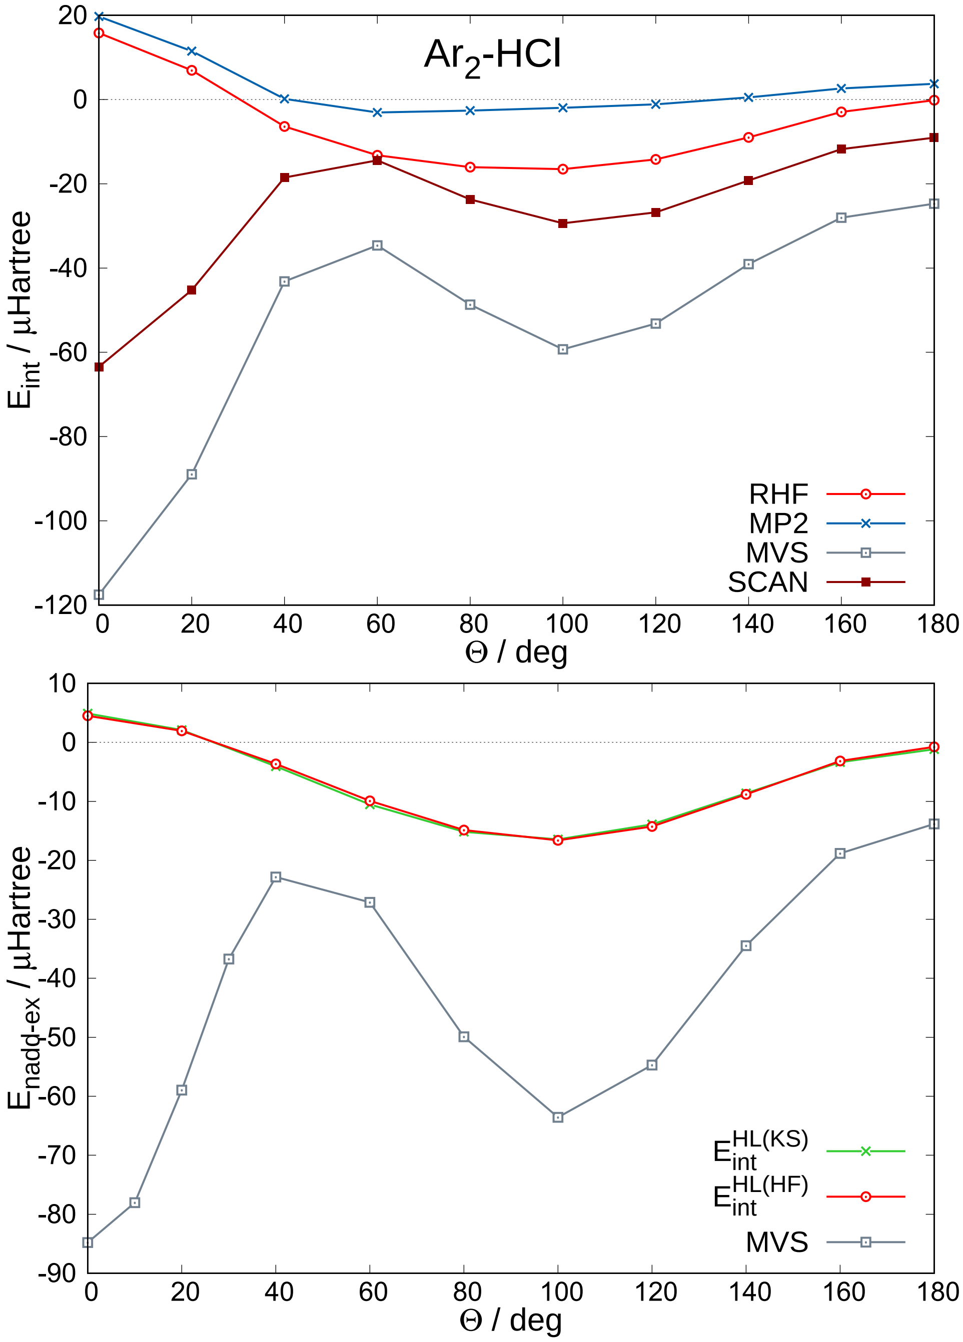


FIG. S4. In-plane bend of $Ar_2$-HCl. Top: total three-body nonadditive interaction energy ($\mu$Hartree), $E_{\mathrm{int}}$. Bottom: three-body nonadditive exchange interaction energy, $E_{\mathrm{nadd-ex}}$ ($\mu$Hartree).

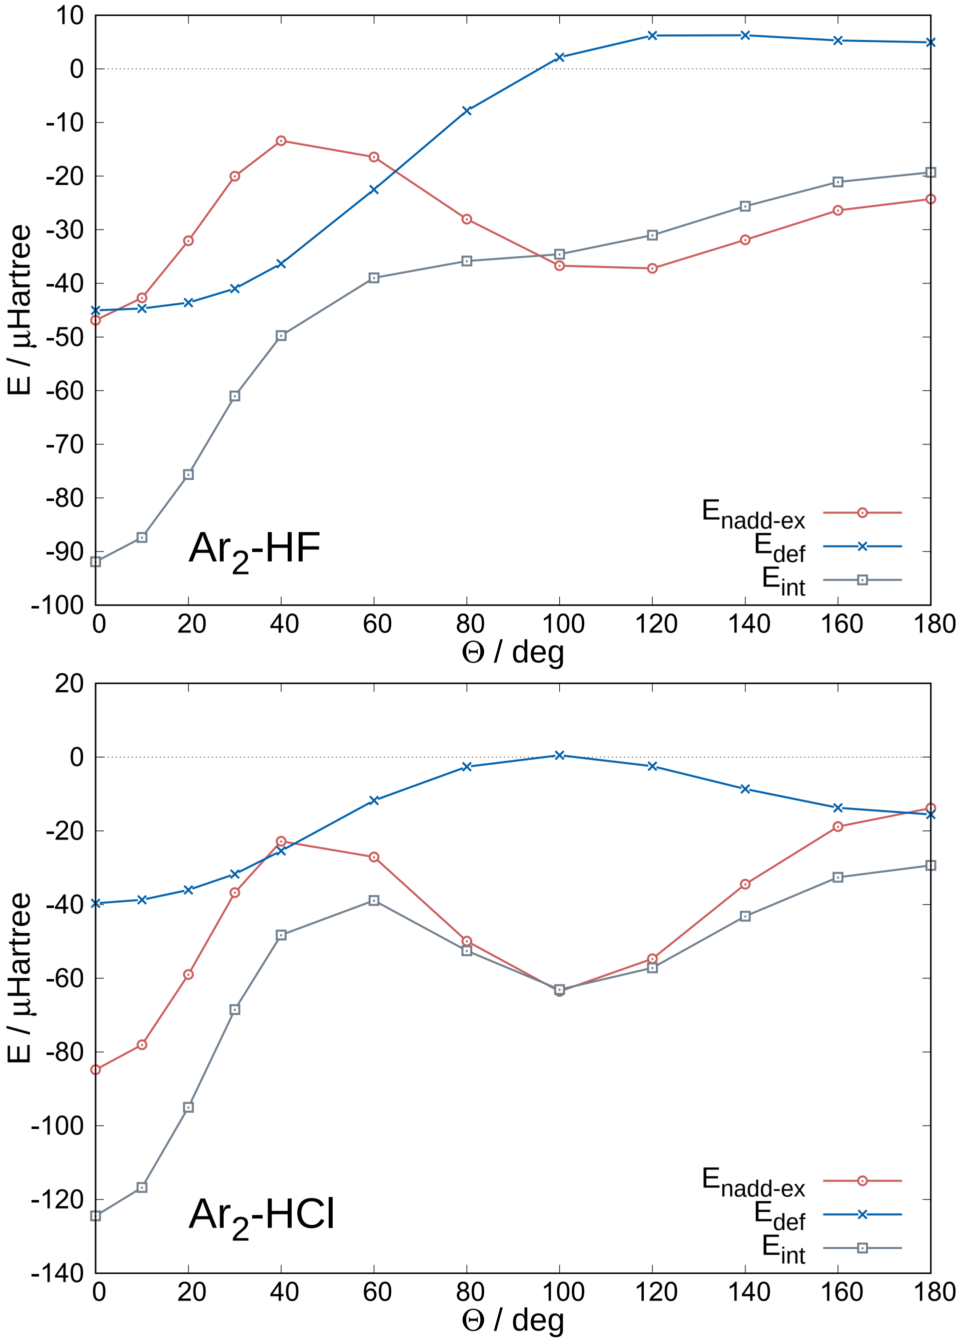


FIG. S5. Decomposition of the supermolecular MVS nonadditive interaction energy ($E_{\rm int} = E_{\rm nadd-ex} + E_{\rm def}$) for the in-plane bend of $Ar_2$-HX Top: $X$ = F, bottom: $X$ = Cl ($\mu$Hartree).

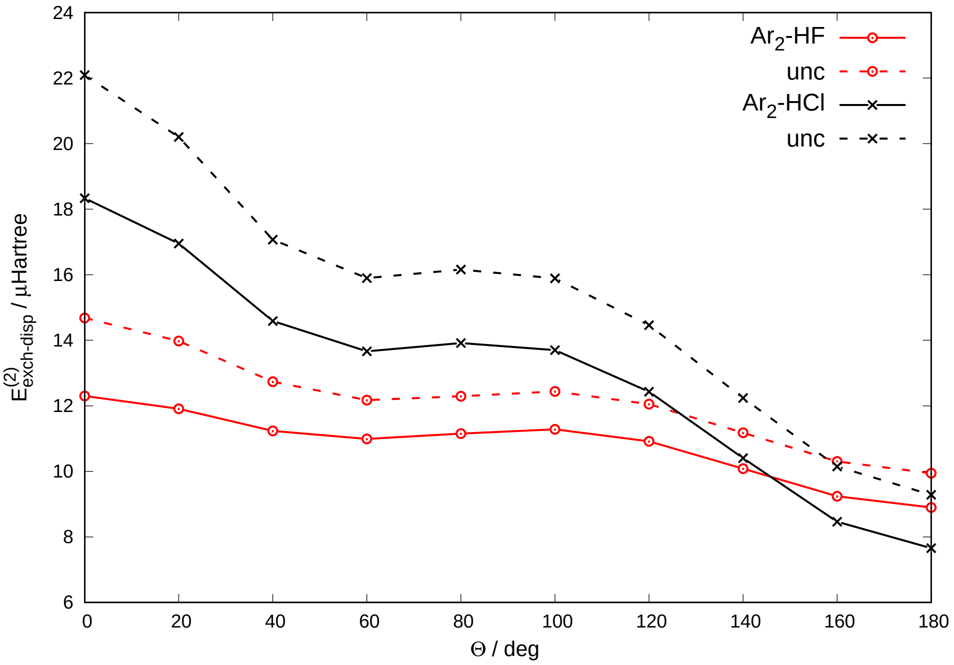


FIG. S6. Three-body nonadditive coupled and uncoupled (unc) second-order exchange-dispersion energy $E^{(2)}_{\mathrm{exch-disp}}$ for the in-plane bend of the $Ar_2$-HF and $Ar_2$-HCl trimers. The results were obtained with the PBE0AC functional and aug-cc-pVQZ basis set.

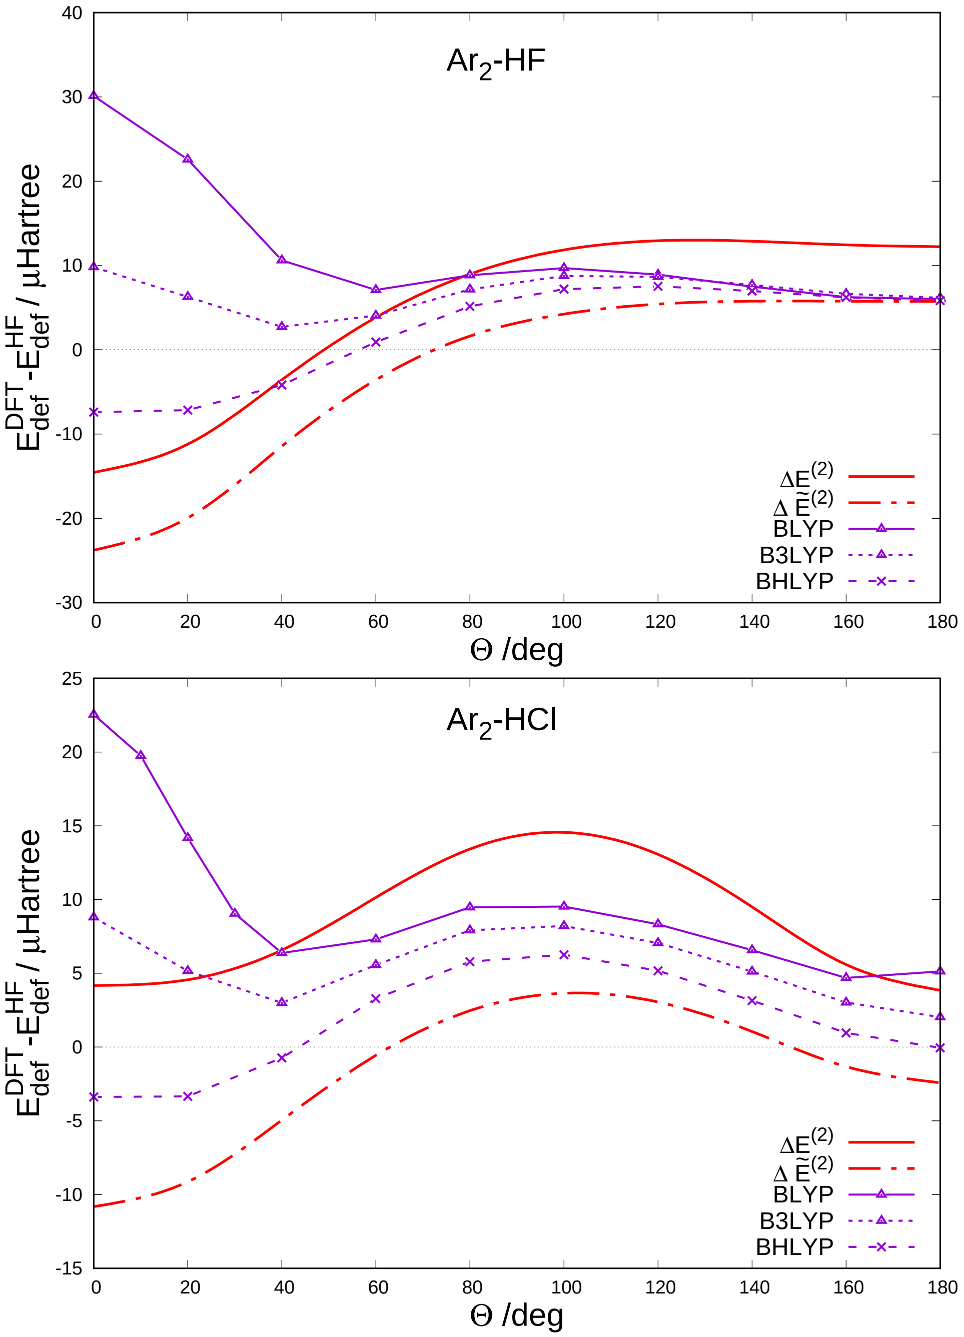


FIG. S7. Difference between the 3-body deformation energy at the DFT and Hartree-Fock levels of theory, $E_{\rm def}^{\rm corr,DFT}$, for the in-plane bend of the Ar$_2$-HX (X = F, Cl) trimers. See the manuscript for definitions of $\Delta E^{(2)}$ and $\Delta\tilde{E}^{(2)}$. The basis set was aug-cc-pVQZ.

TABLE S6: Supermolecular nonadditive three-body interaction energy ($E_{\mathrm{int}}$) and its exchange ($E_{\mathrm{nadd-ex}}$) and deformation ($E_{\mathrm{def}}$) components for $Ar_2$-HX (X = F, Cl) at RHF, PBdf and DFT levels of theory. All energies given in $\mu$Hartree.

| | $Ar_2$-HF | | | $Ar_2$-HCl | | |
|---|---|---|---|---|---|---|
| | | | RHF | | | |
| $\Theta$ | $E_{\mathrm{nadd-ex}}$ | $E_{\mathrm{def}}$ | $E_{\mathrm{int}}$ | $E_{\mathrm{nadd-ex}}$ | $E_{\mathrm{def}}$ | $E_{\mathrm{int}}$ |
| 0 | 25.408 | 31.105 | 56.513 | 4.509 | 11.271 | 15.780 |
| 20 | 20.064 | 19.820 | 39.885 | 1.961 | 4.952 | 6.913 |
| 40 | 8.214 | 0.818 | 9.032 | -3.657 | -2.754 | -6.410 |
| 60 | -3.469 | -7.046 | -10.516 | -9.925 | -3.300 | -13.224 |
| 80 | -11.870 | -4.985 | -16.855 | -14.876 | -1.172 | -16.048 |
| 100 | -16.455 | -0.480 | -16.935 | -16.604 | 0.087 | -16.516 |
| 120 | -17.677 | 2.882 | -14.796 | -14.259 | 0.047 | -14.212 |
| 140 | -16.647 | 4.658 | -11.989 | -8.811 | -0.194 | -9.005 |
| 160 | -14.961 | 5.414 | -9.547 | -3.165 | 0.207 | -2.958 |
| 180 | -14.177 | 5.640 | -8.537 | -0.761 | 0.611 | -0.150 |
| | | | PBdf(PBE0) | | | |
| $\Theta$ | $E_{\mathrm{nadd-ex}}$ | $E_{\mathrm{def}}$ | $E_{\mathrm{int}}$ | $E_{\mathrm{nadd-ex}}$ | $E_{\mathrm{def}}$ | $E_{\mathrm{int}}$ |
| 0 | 28.680 | 32.772 | 61.452 | 7.192 | 12.490 | 19.682 |
| 20 | 22.744 | 20.241 | 42.985 | 3.769 | 5.114 | 8.884 |
| 40 | 9.334 | 0.155 | 9.489 | -3.453 | -3.491 | -6.944 |
| 60 | -4.088 | -7.642 | -11.730 | -10.813 | -3.644 | -14.458 |
| 80 | -13.683 | -5.053 | -18.735 | -15.992 | -1.145 | -17.137 |
| 100 | -18.667 | -0.245 | -18.912 | -17.454 | 0.109 | -17.345 |
| 120 | -19.629 | 3.142 | -16.487 | -14.746 | -0.012 | -14.758 |
| 140 | -17.972 | 4.845 | -13.127 | -9.059 | -0.250 | -9.310 |
| 160 | -15.674 | 5.547 | -10.127 | -3.341 | 0.164 | -3.177 |
| 180 | -14.645 | 5.742 | -8.904 | -0.934 | 0.573 | -0.361 |
| | | | BLYP | | | |
| $\Theta$ | $E_{\mathrm{nadd-ex}}$ | $E_{\mathrm{def}}$ | $E_{\mathrm{int}}$ | $E_{\mathrm{nadd-ex}}$ | $E_{\mathrm{def}}$ | $E_{\mathrm{int}}$ |
| 0 | 13.986 | 61.212 | 75.198 | -20.033 | 33.815 | 13.782 |
| 20 | 3.030 | 42.392 | 45.421 | -29.118 | 19.131 | -9.988 |

| | | | | | | |
|---|---|---|---|---|---|---|
| 40 | -18.188 | 11.434 | -6.754 | -42.825 | 3.628 | -39.198 |
| 60 | -34.782 | 0.045 | -34.737 | -49.234 | 4.006 | -45.228 |
| 80 | -45.495 | 3.849 | -41.646 | -54.970 | 8.297 | -46.673 |
| 100 | -50.883 | 9.206 | -41.677 | -55.961 | 9.616 | -46.345 |
| 120 | -51.915 | 11.805 | -40.110 | -51.073 | 8.368 | -42.705 |
| 140 | -50.355 | 12.146 | -38.209 | -44.999 | 6.377 | -38.622 |
| 160 | -48.458 | 11.658 | -36.800 | -39.781 | 4.896 | -34.886 |
| 180 | -47.687 | 11.648 | -36.039 | -37.991 | 5.744 | -32.246 |

B3LYP

| $\Theta$ | $E_{\mathrm{nadd-ex}}$ | $E_{\mathrm{def}}$ | $E_{\mathrm{int}}$ | $E_{\mathrm{nadd-ex}}$ | $E_{\mathrm{def}}$ | $E_{\mathrm{int}}$ |
|---|---|---|---|---|---|---|
| 0 | 37.395 | 40.902 | 78.297 | 8.626 | 20.069 | 28.695 |
| 20 | 26.937 | 26.087 | 53.025 | -0.470 | 10.108 | 9.638 |
| 40 | 6.347 | 3.525 | 9.872 | -14.938 | 0.239 | -14.699 |
| 60 | -10.124 | -2.995 | -13.119 | -22.412 | 2.261 | -20.151 |
| 80 | -20.517 | 2.178 | -18.339 | -27.724 | 6.748 | -20.976 |
| 100 | -25.855 | 8.284 | -17.571 | -28.885 | 8.295 | -20.591 |
| 120 | -27.500 | 11.535 | -15.965 | -25.575 | 7.102 | -18.473 |
| 140 | -27.017 | 12.350 | -14.668 | -21.427 | 4.930 | -16.497 |
| 160 | -26.084 | 12.052 | -14.033 | -17.950 | 3.233 | -14.717 |
| 180 | -25.696 | 11.802 | -13.893 | -16.801 | 2.642 | -14.159 |

PBE

| $\Theta$ | $E_{\mathrm{nadd-ex}}$ | $E_{\mathrm{def}}$ | $E_{\mathrm{int}}$ | $E_{\mathrm{nadd-ex}}$ | $E_{\mathrm{def}}$ | $E_{\mathrm{int}}$ |
|---|---|---|---|---|---|---|
| 0 | 206.505 | 39.538 | 246.042 | 180.889 | 21.412 | 202.301 |
| 20 | 191.567 | 26.175 | 217.743 | 163.764 | 12.033 | 175.797 |
| 40 | 160.703 | 6.629 | 167.331 | 134.724 | 3.521 | 138.244 |
| 60 | 136.571 | 1.815 | 138.386 | 120.072 | 6.577 | 126.649 |
| 80 | 122.759 | 7.873 | 130.632 | 114.775 | 11.577 | 126.351 |
| 100 | 114.949 | 14.158 | 129.107 | 112.865 | 12.942 | 125.807 |
| 120 | 109.157 | 17.044 | 126.201 | 111.472 | 11.004 | 122.475 |
| 140 | 103.914 | 16.869 | 120.783 | 106.634 | 7.781 | 114.415 |
| 160 | 99.346 | 15.607 | 114.953 | 100.515 | 5.150 | 105.665 |
| 180 | 97.422 | 14.470 | 111.892 | 98.178 | 2.681 | 100.859 |

PBE0

| $\Theta$ | $E_{\mathrm{nadd-ex}}$ | $E_{\mathrm{def}}$ | $E_{\mathrm{int}}$ | $E_{\mathrm{nadd-ex}}$ | $E_{\mathrm{def}}$ | $E_{\mathrm{int}}$ |
|---|---|---|---|---|---|---|
| 0 | 136.595 | 22.338 | 158.933 | 116.237 | 9.025 | 125.262 |
| 20 | 125.227 | 12.222 | 137.449 | 104.054 | 3.078 | 107.133 |
| 40 | 100.945 | -1.428 | 99.517 | 82.914 | -1.614 | 81.300 |
| 60 | 81.509 | -3.609 | 77.900 | 71.159 | 1.859 | 73.017 |
| 80 | 70.115 | 2.768 | 72.882 | 66.281 | 6.481 | 72.762 |
| 100 | 63.947 | 9.279 | 73.226 | 64.813 | 8.000 | 72.813 |
| 120 | 60.282 | 12.766 | 73.048 | 64.996 | 6.560 | 71.556 |
| 140 | 57.916 | 13.326 | 71.242 | 63.544 | 3.936 | 67.479 |
| 160 | 56.109 | 12.705 | 68.814 | 61.138 | 1.863 | 63.001 |
| 180 | 55.352 | 12.157 | 67.509 | 60.551 | -0.724 | 59.827 |

$\omega$PBE

| $\Theta$ | $E_{\mathrm{nadd-ex}}$ | $E_{\mathrm{def}}$ | $E_{\mathrm{int}}$ | $E_{\mathrm{nadd-ex}}$ | $E_{\mathrm{def}}$ | $E_{\mathrm{int}}$ |
|---|---|---|---|---|---|---|
| 0 | 2.134 | -2.389 | -0.255 | -18.540 | -9.680 | -28.220 |
| 20 | -2.121 | -7.378 | -9.499 | -20.044 | -10.415 | -30.460 |
| 40 | -13.792 | -13.232 | -27.023 | -23.695 | -9.036 | -32.730 |
| 60 | -25.507 | -10.935 | -36.442 | -30.533 | -4.190 | -34.723 |
| 80 | -34.197 | -3.032 | -37.228 | -35.945 | 0.359 | -35.585 |
| 100 | -38.702 | 4.091 | -34.611 | -37.578 | 2.196 | -35.383 |
| 120 | -38.822 | 8.160 | -30.662 | -33.996 | 1.335 | -32.661 |
| 140 | -35.438 | 9.638 | -25.800 | -27.049 | -0.744 | -27.794 |
| 160 | -31.380 | 9.902 | -21.478 | -19.853 | -2.264 | -22.117 |
| 180 | -29.517 | 9.951 | -19.566 | -15.802 | -2.827 | -18.630 |

LC-PBETPSS

| $\Theta$ | $E_{\mathrm{nadd-ex}}$ | $E_{\mathrm{def}}$ | $E_{\mathrm{int}}$ | $E_{\mathrm{nadd-ex}}$ | $E_{\mathrm{def}}$ | $E_{\mathrm{int}}$ |
|---|---|---|---|---|---|---|
| 0 | -2.060 | -0.123 | -2.182 | -28.279 | -11.353 | -39.632 |
| 20 | -7.122 | -6.387 | -13.508 | -28.617 | -11.780 | -40.397 |
| 40 | -20.887 | -13.986 | -34.873 | -30.815 | -9.840 | -40.655 |
| 60 | -35.073 | -11.776 | -46.848 | -37.821 | -4.592 | -42.414 |
| 80 | -45.473 | -3.110 | -48.583 | -43.729 | 0.218 | -43.511 |
| 100 | -50.573 | 4.688 | -45.885 | -45.538 | 2.175 | -43.363 |

| | | | | | | |
|---|---|---|---|---|---|---|
| 120 | -50.271 | 9.111 | -41.160 | -41.496 | 1.277 | -40.219 |
| 140 | -45.832 | 10.671 | -35.161 | -33.386 | -0.920 | -34.306 |
| 160 | -40.658 | 10.874 | -29.784 | -24.924 | -2.537 | -27.461 |
| 180 | -38.360 | 11.310 | -28.956 | -20.257 | -3.132 | -23.389 |

TABLE S7: Supermolecular ($E_{\rm int}$) and PBdf ($E^{\rm dfree}_{\rm int}$) three-body nonadditive interaction energies for dispersion-bound trimers: $N_2$, CO and $CH_4$ ($\mu$Hartree) and hydrogen-bound trimers: HF and $NH_3$ (kcal/mol). Geometries taken from Ref. 12. All DFT calculations in the aug-cc-pVTZ basis set. The MP2 and CCSD(T) energies were extrapolated (aug-cc-pVTZ → aug-cc-pVQZ) using the formula of Halkier *et al.*[13].

| $\mathbf{N_2}$ | $E_{\rm nadd-ex}$ | $E^{\rm dfree}_{\rm nadd-ex}$ | $E_{\rm def}$ | $E^{\rm dfree}_{\rm def}$ | $E_{\rm int}$ | $E^{\rm dfree}_{\rm int}$ |
|---|---|---|---|---|---|---|
| HF | -4.031 | -4.031 | -3.662 | -3.662 | -7.693 | -7.693 |
| PBE | 49.85 | -4.496 | -2.176 | -6.636 | 80.00 | -11.13 |
| PBE0 | 82.17 | -3.949 | -4.120 | -5.295 | 45.73 | -9.245 |
| BLYP | -38.88 | -2.863 | -2.559 | -7.368 | -41.44 | -10.23 |
| BHLYP | -9.988 | -3.407 | -4.328 | -6.636 | -14.32 | -8.164 |
| MVS | -10.84 | -2.552 | -23.39 | -4.978 | -32.24 | -7.530 |
| $\omega$PBE | -17.92 | -3.859 | -8.792 | -6.631 | -26.71 | -10.49 |
| $\omega$B97XD3 | | | | | -20.24 | |
| $E^{(2;0)}_{\rm exch-disp}(S^2+S^3)$ | | | | | 6.082 | |
| MP2 | | | | | -3.744 | |
| CCSD(T) | | | | | 4.086 | |
| **CO** | $E_{\rm nadd-ex}$ | $E^{\rm dfree}_{\rm nadd-ex}$ | $E_{\rm def}$ | $E^{\rm dfree}_{\rm def}$ | $E_{\rm int}$ | $E^{\rm dfree}_{\rm int}$ |
| HF | -12.86 | -12.86 | 1.205 | 1.205 | -11.66 | -11.66 |
| PBE | 100.0 | -21.86 | 7.470 | 2.341 | 107.5 | -19.52 |
| PBE0 | 57.60 | -17.68 | 3.391 | 1.866 | 61.00 | -15.81 |
| BLYP | -60.15 | -18.82 | 7.722 | 2.167 | -52.43 | -16.65 |
| BHLYP | -17.65 | -14.90 | 2.367 | 1.865 | -15.28 | -13.49 |
| MVS | -124.9 | -13.56 | -1.258 | 3.583 | -126.2 | -9.977 |
| $\omega$PBE | -33.70 | -15.51 | -2.705 | 2.055 | -36.41 | -13.46 |
| $\omega$B97XD3 | | | | | -28.91 | |
| $E^{(2;0)}_{\rm exch-disp}(S^2+S^3)$ | | | | | 8.939 | |
| MP2 | | | | | -9.304 | |

| CCSD(T) | | | | | 5.808 | |
|---|---|---|---|---|---|---|

| $\mathbf{CH_4}$ | $E_{\text{nadd-ex}}$ | $E^{\text{dfree}}_{\text{nadd-ex}}$ | $E_{\text{def}}$ | $E^{\text{dfree}}_{\text{def}}$ | $E_{\text{int}}$ | $E^{\text{dfree}}_{\text{int}}$ |
|---|---|---|---|---|---|---|
| HF | -20.40 | -20.40 | -0.819 | -0.819 | -21.22 | -21.22 |
| PBE | 176.5 | -26.40 | 10.84 | -0.908 | 187.4 | -27.31 |
| PBE0 | 101.8 | -24.17 | 3.976 | -1.149 | 105.8 | -25.32 |
| BLYP | -69.24 | -21.94 | 11.73 | -0.534 | -57.51 | -22.48 |
| BHLYP | -8.696 | -21.61 | 3.541 | -0.740 | -5.155 | -22.35 |
| MVS | -187.7 | -20.13 | -16.22 | -1.639 | -204.0 | -21.77 |
| $\omega$PBE | -70.16 | -24.63 | -10.07 | -1.900 | -80.23 | -26.53 |
| $\omega$B97XD3 | | | | | -52.71 | |
| $E^{(2;0)}_{\text{exch-disp}}(S^2+S^3)$ | | | | | 20.604 | |
| MP2 | | | | | -5.241 | |
| CCSD(T) | | | | | 24.66 | |

| **HF** | $E_{\text{nadd-ex}}$ | $E^{\text{dfree}}_{\text{nadd-ex}}$ | $E_{\text{def}}$ | $E^{\text{dfree}}_{\text{def}}$ | $E_{\text{int}}$ | $E^{\text{dfree}}_{\text{int}}$ |
|---|---|---|---|---|---|---|
| HF | -0.383 | -0.383 | -3.711 | -3.711 | -4.094 | -4.094 |
| PBE | 0.149 | -0.341 | -4.478 | -4.279 | -4.329 | -4.620 |
| PBE0 | -0.024 | -0.366 | -4.238 | -4.049 | -4.262 | -4.415 |
| BLYP | -0.112 | -0.331 | -4.464 | -4.176 | -4.576 | -4.507 |
| BHLYP | -0.008 | -0.396 | -4.011 | -3.764 | -4.019 | -4.160 |
| MVS | -0.182 | -0.378 | -4.237 | -3.946 | -4.419 | -4.324 |
| $\omega$PBE | -0.386 | -0.389 | -4.020 | -3.805 | -4.407 | -4.194 |
| $\omega$B97XD3 | | | | | -4.512 | |
| $E^{(2;0)}_{\text{exch-disp}}(S^2+S^3)$ | | | | | 0.107 | |
| MP2 | | | | | -4.218 | |
| CCSD(T) | | | | | -4.176 | |

| $\mathbf{NH_3}$ | $E_{\text{nadd-ex}}$ | $E^{\text{dfree}}_{\text{nadd-ex}}$ | $E_{\text{def}}$ | $E^{\text{dfree}}_{\text{def}}$ | $E_{\text{int}}$ | $E^{\text{dfree}}_{\text{int}}$ |
|---|---|---|---|---|---|---|
| HF | -0.107 | -0.107 | -1.106 | -1.106 | -1.213 | -1.213 |
| PBE | 0.264 | -0.052 | -1.442 | -1.150 | -1.177 | -1.203 |
| PBE0 | 0.142 | -0.078 | -1.346 | -1.132 | -1.204 | -1.210 |
| BLYP | -0.005 | -0.035 | -1.416 | -1.142 | -1.421 | -1.177 |
| BHLYP | 0.056 | -0.093 | -1.250 | -1.083 | -1.194 | -1.177 |
| MVS | -0.145 | -0.081 | -1.321 | -1.144 | -1.466 | -1.225 |
| $\omega$PBE | -0.113 | -0.120 | -1.281 | -1.120 | -1.394 | -1.240 |

| | |
|---|---|
| ωB97XD3 | -1.332 |
| $E^{(2;0)}_{\mathrm{exch-disp}}(S^2 + S^3)$ | 0.109 |
| MP2 | -1.191 |
| CCSD(T) | -1.151 |

TABLE S8: Supermolecular ($E_{\mathrm{int}}$) and PBdf ($E^{\mathrm{dfree}}_{\mathrm{int}}$) three-body nonadditive energies (kcal/mol) for trimers of the 3B-69 basis: **1** - water, **2** - formaldehyde, **3** - methanol-ethyne, **4** - acetonitrile. Geometries, MP2/CBS, CCSD(T)/CBS and $E^{\mathrm{AIFF}}_{\mathrm{disp}}$ values taken taken from Ref. 11. PBdf and $E^{(2;0)}_{\mathrm{exch-disp}}(S^2 + S^3)$ calculations performed in the aug-cc-pVTZ basis set.

| | $E_{\mathrm{nadd-ex}}$ | $E^{\mathrm{dfree}}_{\mathrm{nadd-ex}}$ | $E_{\mathrm{def}}$ | $E^{\mathrm{dfree}}_{\mathrm{def}}$ | $E_{\mathrm{int}}$ | $E^{\mathrm{dfree}}_{\mathrm{int}}$ | $E^{\mathrm{AIFF}}_{\mathrm{disp}}$ |
|---|---|---|---|---|---|---|---|
| **1a** | | | | | | | |
| HF | -0.063 | -0.063 | -1.333 | -1.333 | -1.396 | -1.396 | 0.002 |
| PBE | 0.036 | -0.045 | -1.494 | -1.420 | -1.458 | -1.466 | |
| PBE0 | -0.003 | -0.054 | -1.452 | -1.384 | -1.455 | -1.437 | |
| BLYP | -0.112 | -0.040 | -1.492 | -1.399 | -1.604 | -1.439 | |
| BHLYP | -0.072 | -0.056 | -1.403 | -1.323 | -1.475 | -1.379 | |
| MVS | -0.036 | -0.059 | -1.435 | -1.362 | -1.471 | -1.421 | |
| ωPBE | -0.044 | -0.046 | -1.422 | -1.342 | -1.467 | -1.388 | |
| ωB97XD3 | | | | | -1.461 | | |
| $E^{(2;0)}_{\mathrm{exch-disp}}(S^2 + S^3)$ | 0.032 | | | | | | |
| MP2 | -1.392 | | | | | | |
| CCSD(T) | -1.386 | | | | | | |
| **1b** | | | | | | | |
| HF | -0.132 | -0.132 | 1.118 | 1.118 | 0.986 | 0.986 | 0.004 |
| PBE | -0.012 | -0.115 | 1.343 | 1.182 | 1.331 | 1.067 | |
| PBE0 | -0.054 | -0.122 | 1.287 | 1.155 | 1.233 | 1.033 | |
| BLYP | -0.188 | -0.112 | 1.294 | 1.173 | 1.106 | 1.061 | |
| BHLYP | -0.131 | -0.127 | 1.217 | 1.110 | 1.086 | 0.982 | |
| MVS | -0.113 | -0.117 | 1.356 | 1.136 | 1.244 | 1.019 | |
| ωPBE | -0.138 | -0.144 | 1.249 | 1.126 | 1.111 | 0.983 | |
| ωB97XD3 | | | | | 1.167 | | |
| $E^{(2;0)}_{\mathrm{exch-disp}}(S^2 + S^3)$ | 0.052 | | | | | | |
| MP2 | 1.068 | | | | | | |

| | | | | | | | |
|---|---|---|---|---|---|---|---|
| CCSD(T) | 1.084 | | | | | | |
| **1c** | | | | | | | |
| HF | -0.286 | -0.286 | -2.187 | -2.187 | -2.473 | -2.473 | 0.028 |
| PBE | 0.217 | -0.225 | -2.665 | -2.395 | -2.449 | -2.620 | |
| PBE0 | 0.058 | -0.252 | -2.524 | -2.308 | -2.466 | -2.560 | |
| BLYP | -0.079 | -0.210 | -2.655 | -2.350 | -2.734 | -2.560 | |
| BHLYP | 0.002 | -0.278 | -2.392 | -2.175 | -2.389 | -2.453 | |
| MVS | -0.175 | -0.257 | -2.492 | -2.270 | -2.668 | -2.527 | |
| $\omega$PBE | -0.273 | -0.286 | -2.417 | -2.219 | -2.692 | -2.505 | |
| $\omega$B97XD3 | | | | | -2.686 | | |
| $E^{(2;0)}_{\mathrm{exch-disp}}(S^2+S^3)$ | 0.127 | | | | | | |
| MP2 | -2.472 | | | | | | |
| CCSD(T) | -2.416 | | | | | | |

| | $E_{\mathrm{nadd-ex}}$ | $E^{\mathrm{dfree}}_{\mathrm{nadd-ex}}$ | $E_{\mathrm{def}}$ | $E^{\mathrm{dfree}}_{\mathrm{def}}$ | $E_{\mathrm{int}}$ | $E^{\mathrm{dfree}}_{\mathrm{int}}$ | $E^{\mathrm{AIFF}}_{\mathrm{disp}}$ |
|---|---|---|---|---|---|---|---|
| **2a** | | | | | | | |
| HF | -0.001 | -0.001 | -0.235 | -0.235 | -0.236 | -0.236 | -0.001 |
| PBE | -0.002 | -0.002 | -0.168 | -0.166 | -0.169 | -0.168 | |
| PBE0 | -0.001 | -0.001 | -0.184 | -0.182 | -0.185 | -0.183 | |
| BLYP | -0.002 | -0.001 | -0.173 | -0.174 | -0.175 | -0.176 | |
| BHLYP | -0.001 | -0.001 | -0.206 | -0.205 | -0.208 | -0.207 | |
| MVS | -0.001 | -0.001 | -0.178 | -0.175 | -0.179 | -0.176 | |
| $\omega$PBE | -0.001 | -0.001 | -0.203 | -0.199 | -0.204 | -0.200 | |
| $\omega$B97XD3 | | | | | -0.197 | | |
| $E^{(2;0)}_{\mathrm{exch-disp}}(S^2+S^3)$ | 0.000 | | | | | | |
| MP2 | -0.168 | | | | | | |
| CCSD(T) | -0.178 | | | | | | |
| **2b** | | | | | | | |
| HF | -0.075 | -0.075 | 0.250 | 0.250 | 0.176 | 0.176 | 0.020 |
| PBE | 0.110 | -0.080 | 0.195 | 0.194 | 0.305 | 0.114 | |
| PBE0 | 0.047 | -0.076 | 0.211 | 0.198 | 0.258 | 0.122 | |
| BLYP | -0.097 | -0.079 | 0.202 | 0.198 | 0.105 | 0.119 | |
| BHLYP | -0.033 | -0.078 | 0.231 | 0.226 | 0.198 | 0.148 | |
| MVS | -0.104 | -0.061 | 0.182 | 0.187 | 0.078 | 0.126 | |

| | | | | | | | |
|---|---|---|---|---|---|---|---|
| $\omega$PBE | -0.107 | -0.080 | 0.223 | 0.219 | 0.115 | 0.139 | |
| $\omega$B97XD3 | | | | | 0.125 | | |
| $E^{(2;0)}_{\mathrm{exch-disp}}(S^2+S^3)$ | 0.032 | | | | | | |
| MP2 | 0.161 | | | | | | |
| CCSD(T) | 0.181 | | | | | | |
| **2c** | | | | | | | |
| HF | 0.009 | 0.009 | -0.145 | -0.145 | -0.136 | -0.136 | 0.013 |
| PBE | 0.147 | 0.004 | -0.135 | -0.110 | 0.012 | -0.106 | |
| PBE0 | 0.096 | 0.006 | -0.140 | -0.116 | -0.045 | -0.110 | |
| BLYP | -0.012 | 0.007 | -0.131 | -0.119 | -0.143 | -0.112 | |
| BHLYP | 0.028 | 0.008 | -0.145 | -0.129 | -0.118 | -0.121 | |
| MVS | -0.140 | 0.003 | -0.173 | -0.100 | -0.314 | -0.097 | |
| $\omega$PBE | -0.006 | 0.008 | -0.158 | -0.123 | -0.164 | -0.115 | |
| $\omega$B97XD3 | | | | | -0.181 | | |
| $E^{(2;0)}_{\mathrm{exch-disp}}(S^2+S^3)$ | 0.014 | | | | | | |
| MP2 | -0.095 | | | | | | |
| CCSD(T) | -0.093 | | | | | | |

| | $E_{\mathrm{nadd-ex}}$ | $E^{\mathrm{dfree}}_{\mathrm{nadd-ex}}$ | $E_{\mathrm{def}}$ | $E^{\mathrm{dfree}}_{\mathrm{def}}$ | $E_{\mathrm{int}}$ | $E^{\mathrm{dfree}}_{\mathrm{int}}$ | $E^{\mathrm{AIFF}}_{\mathrm{disp}}$ |
|---|---|---|---|---|---|---|---|
| **3a** | | | | | | | |
| HF | -0.051 | -0.051 | -1.215 | -1.215 | -1.265 | -1.265 | 0.016 |
| PBE | 0.052 | -0.047 | -1.432 | -1.368 | -1.380 | -1.415 | |
| PBE0 | 0.008 | -0.054 | -1.366 | -1.302 | -1.358 | -1.357 | |
| BLYP | -0.127 | -0.031 | -1.430 | -1.355 | -1.557 | -1.386 | |
| BHLYP | -0.069 | -0.046 | -1.306 | -1.223 | -1.375 | -1.268 | |
| MVS | -0.043 | -0.067 | -1.362 | -1.270 | -1.405 | -1.337 | |
| $\omega$PBE | -0.040 | -0.036 | -1.322 | -1.235 | -1.362 | -1.271 | |
| $\omega$B97XD3 | | | | | -1.374 | | |
| $E^{(2;0)}_{\mathrm{exch-disp}}(S^2+S^3)$ | 0.052 | | | | | | |
| MP2 | -1.305 | | | | | | |
| CCSD(T) | -1.308 | | | | | | |
| **3b** | | | | | | | |
| HF | -0.004 | -0.004 | 0.034 | 0.034 | 0.030 | 0.030 | 0.015 |
| PBE | 0.077 | -0.003 | 0.036 | 0.030 | 0.113 | 0.028 | |

| | | | | | | | |
|---|---|---|---|---|---|---|---|
| PBE0 | 0.047 | -0.003 | 0.033 | 0.031 | 0.080 | 0.027 | |
| BLYP | -0.035 | -0.001 | 0.037 | 0.030 | 0.002 | 0.029 | |
| BHLYP | -0.008 | -0.003 | 0.034 | 0.033 | 0.026 | 0.030 | |
| MVS | -0.052 | -0.003 | 0.019 | 0.030 | 0.033 | 0.027 | |
| $\omega$PBE | -0.014 | -0.003 | 0.029 | 0.032 | 0.014 | 0.029 | |
| $\omega$B97XD3 | | | | | 0.027 | | |
| $E^{(2;0)}_{\text{exch-disp}}(S^2+S^3)$ | 0.008 | | | | | | |
| MP2 | 0.036 | | | | | | |
| CCSD(T) | 0.047 | | | | | | |
| **3c** | | | | | | | |
| HF | 0.059 | 0.059 | -0.081 | -0.081 | -0.021 | -0.021 | 0.018 |
| PBE | 0.201 | 0.069 | -0.091 | -0.075 | 0.110 | -0.006 | |
| PBE0 | 0.148 | 0.064 | -0.095 | -0.077 | 0.053 | -0.013 | |
| BLYP | 0.031 | 0.074 | -0.086 | -0.075 | -0.055 | -0.001 | |
| BHLYP | 0.072 | 0.064 | -0.093 | -0.075 | -0.021 | -0.012 | |
| MVS | 0.036 | 0.060 | -0.110 | -0.074 | -0.073 | -0.014 | |
| $\omega$PBE | 0.048 | 0.059 | -0.096 | -0.075 | -0.048 | -0.017 | |
| $\omega$B97XD3 | | | | | -0.035 | | |
| $E^{(2;0)}_{\text{exch-disp}}(S^2+S^3)$ | 0.020 | | | | | | |
| MP2 | -0.003 | | | | | | |
| CCSD(T) | 0.023 | | | | | | |

| | $E_{\text{nadd-ex}}$ | $E^{\text{dfree}}_{\text{nadd-ex}}$ | $E_{\text{def}}$ | $E^{\text{dfree}}_{\text{def}}$ | $E_{\text{int}}$ | $E^{\text{dfree}}_{\text{int}}$ | $E^{\text{AIFF}}_{\text{disp}}$ |
|---|---|---|---|---|---|---|---|
| **4a** | | | | | | | |
| HF | -0.023 | -0.023 | 0.223 | 0.223 | 0.200 | 0.200 | 0.052 |
| PBE | 0.198 | -0.026 | 0.228 | 0.206 | 0.426 | 0.180 | |
| PBE0 | 0.117 | -0.024 | 0.216 | 0.210 | 0.333 | 0.186 | |
| BLYP | -0.054 | -0.020 | 0.232 | 0.201 | 0.178 | 0.181 | |
| BHLYP | 0.017 | -0.022 | 0.222 | 0.212 | 0.239 | 0.190 | |
| MVS | -0.129 | -0.021 | 0.156 | 0.213 | 0.027 | 0.193 | |
| $\omega$PBE | -0.081 | -0.026 | 0.180 | 0.213 | 0.099 | 0.187 | |
| $\omega$B97XD3 | | | | | 0.137 | | |
| $E^{(2;0)}_{\text{exch-disp}}(S^2+S^3)$ | 0.040 | | | | | | |
| MP2 | 0.198 | | | | | | |

| | | | | | | | |
|---|---|---|---|---|---|---|---|
| CCSD(T) | 0.254 | | | | | | |
| **4b** | | | | | | | |
| HF | -0.041 | -0.041 | 0.357 | 0.357 | 0.316 | 0.316 | 0.019 |
| PBE | 0.062 | -0.046 | 0.391 | 0.348 | 0.454 | 0.301 | |
| PBE0 | 0.028 | -0.042 | 0.376 | 0.344 | 0.404 | 0.301 | |
| BLYP | -0.083 | -0.045 | 0.389 | 0.359 | 0.306 | 0.314 | |
| BHLYP | -0.037 | -0.042 | 0.371 | 0.351 | 0.333 | 0.309 | |
| MVS | -0.100 | -0.036 | 0.380 | 0.344 | 0.280 | 0.308 | |
| $\omega$PBE | -0.054 | -0.042 | 0.360 | 0.339 | 0.306 | 0.297 | |
| $\omega$B97XD3 | | | | | 0.341 | | |
| $E^{(2;0)}_{\mathrm{exch-disp}}(S^2+S^3)$ | 0.023 | | | | | | |
| MP2 | 0.319 | | | | | | |
| CCSD(T) | 0.335 | | | | | | |
| **4c** | | | | | | | |
| HF | 0.014 | 0.014 | -0.191 | -0.191 | -0.177 | -0.177 | -0.004 |
| PBE | 0.016 | 0.016 | -0.191 | -0.175 | -0.175 | -0.159 | |
| PBE0 | 0.014 | 0.014 | -0.190 | -0.177 | -0.176 | -0.163 | |
| BLYP | 0.014 | 0.017 | -0.184 | -0.177 | -0.170 | -0.160 | |
| BHLYP | 0.013 | 0.015 | -0.191 | -0.182 | -0.178 | -0.167 | |
| MVS | 0.011 | 0.011 | -0.196 | -0.181 | -0.182 | -0.170 | |
| $\omega$PBE | 0.013 | 0.013 | -0.187 | -0.177 | -0.175 | -0.164 | |
| $\omega$B97XD3 | | | | | -0.185 | | |
| $E^{(2;0)}_{\mathrm{exch-disp}}(S^2+S^3)$ | 0.002 | | | | | | |
| MP2 | -0.155 | | | | | | |
| CCSD(T) | -0.166 | | | | | | |

TABLE S9. Mean absolute errors (kcal/mol) with respect to $E_{\rm int}$(CCSD(T)) for the set of 17 trimers. $E^{\rm D3}_{\rm disp}$ denotes the D3 dispersion three-body term based on a damped Axilrod-Teller-Muto (ATM) formula;[14] $E^{(2;0)}_{\rm exch-disp}$ is the nonadditive second-order exchange-dispersion energy obtained at the uncoupled Hartree-Fock level in the $S^2 + S^3$ approximation.

| | HF | BLYP | BHLYP | PBE | PBE0 | $\omega$PBE | $\omega$B97XD3 | MP2 |
|---|---|---|---|---|---|---|---|---|
| $E_{\rm int}$+$E^{\rm D3}_{\rm disp}$ | 0.032 | 0.108 | 0.032 | 0.093 | 0.058 | 0.079 | 0.087 | 0.020 |
| $E_{\rm int}$+$E^{\rm D3}_{\rm disp}$+$E^{(2;0)}_{\rm exch-disp}$ | **0.043** | **0.080** | **0.052** | **0.100** | **0.073** | **0.053** | **0.058** | |
| $E^{\rm dfree}_{\rm int}$+$E^{\rm D3}_{\rm disp}$ | 0.032 | 0.046 | 0.024 | 0.063 | 0.044 | 0.031 | | |
| $E^{\rm dfree}_{\rm int}$+$E^{\rm D3}_{\rm disp}$+$E^{(2;0)}_{\rm exch-disp}$ | **0.043** | **0.030** | **0.038** | **0.044** | **0.020** | **0.026** | | |
| $E_{\rm int}$-$E^{(2;0)}_{\rm exch-disp}$ | | | | | | | | **0.059** |

## REFERENCES


[1] B. Jeziorski, M. Bulski, and L. Piela, Int. J. Quant. Chem. **10**, 281 (1976).

[2] Ł. Rajchel, P. S. Żuchowski, M. M. Szczęśniak, and G. Chałasiński, Chem. Phys. Lett. **486**, 160 (2010).

[3] Ł. Rajchel, P. S. Żuchowski, M. M. Szczęśniak, and G. Chałasiński, Phys. Rev. Lett. **104**, 163001 (2010).

[4] P.-O. Löwdin, J. Chem. Phys. **18**, 365 (1950).

[5] M. Modrzejewski, Ł. Rajchel, M. M. Szczęśniak, and G. Chałasiński, J. Chem. Phys. **136**, 204109 (2012).

[6] E. Fermi and G. Amaldi, Mem. Accad. Italia **6** (1934).

[7] D. J. Tozer and N. C. Handy, J. Chem. Phys. **109**, 10180 (1998).

[8] R. Bukowski, W. Cencek, P. Jankowski, M. Jeziorska, B. Jeziorski, S. A. Kucharski, V. F. Lotrich, A. J. Misquitta, R. Moszyński, K. Patkowski, R. Podeszwa, S. Rybak, K. Szalewicz, H. L. Williams, R. J. Wheatley, P. E. S. Wormer, and P. S. Żuchowski, "SAPT2012: an ab initio program for many-body symmetry-adapted perturbation theory calculations of intermolecular interaction energies," .

[9] D. E. Woon and T. H. Dunning Jr, J. Chem. Phys. **100**, 2975 (1994).

[10] D. E. Woon and T. H. Dunning Jr, J. Chem. Phys. **98**, 1358 (1993).

[11] J. Řezáč, Y. Huang, P. Hobza, and G. J. Beran, J. Chem. Theory Comput. **11**, 3065 (2015).

[12] A. Otero-de-la Roza, G. A. DiLabio, and E. R. Johnson, J. Chem. Theory Comput. **12**, 3160 (2016).

[13] A. Halkier, W. Klopper, T. Helgaker, P. Jørgensen, and P. R. Taylor, J. Chem. Phys. **111**,

9157 (1999).

[14]S. Grimme, J. Antony, S. Ehrlich, and H. Krieg, J. Chem. Phys. **132**, 154104 (2010).
